# Supplementary material for: Theory for identification and Inference with Synthetic Controls: A Proximal Causal Inference Framework
Source: arXiv:2108.13935 source file (2023-02-18)
Supplement: Supplementary file 1 [file Supplementary_Materials.pdf]

# Supplementary Material for "Theory for Identification and Inference With Synthetic Controls: A Proximal Causal Inference Framework"

February 18, 2023

**This supplement includes extensions of the proximal inference approach to synthetic control, additional simulation studies, and proofs of all theorems.**

# A A conformal inference method for pointwise confidence intervals of ATT

## A.1 Method overview

After obtaining estimates of synthetic control weights, the parametric modeling approach in Section 3.2 applies to the setting where $T_1$ is relatively large so that it is possible to leverage the outcomes at other post-treatment periods to estimate each $\tau_t = E[Y_t(1) - Y_t(0)]$, $t > T_0$. When $T_1$ is small, however, the large-$T_1$ asymptotics considered in Section 3.2 may be inappropriate and the GMM approach may produce invalid inference.

Under the setting where $T_1$ is fixed as $T \to \infty$ and a linear interactive fixed effects model;, Chernozhukov et al. (2021) proposed a conformal inference method to construct pointwise prediction intervals for the treatment effects $\eta_t = Y_t(1) - Y_t(0)$ on the treatment unit by inverting permutation tests. When the treatment effects are considered fixed, their method equivalently produces confidence intervals for the ATT $\tau_t = E[Y_t(1) - Y_t(0)]$. Their framework is general and can be adapted to procedures that produce "mean-unbiased proxies" of $Y_t(0)$. Recall that under Assumptions 1-3, $\sum_{i \in \mathcal{D}} \alpha_i W_{it}$ is a mean-unbiased proxy that satisfies $E[Y_t(0)] = E[\sum_{i \in \mathcal{D}} \alpha_i W_{it}]$ for every $t \geq 1$. Therefore, valid prediction inference for $\eta_t$ is possible using the method in Chernozhukov et al. (2021) with minor modifications. For the rest of the section, we present the conformal inference approach, modified from Chernozhukov et al. (2021), to construct pointwise prediction intervals for $\eta_t$, $t = T_0 + 1, \ldots, T$. We refer the readers to Theorem 1 of Chernozhukov et al. (2021) for the coverage guarantee of the proposed prediction intervals when $T_0$ is large.

For each post-treatment time period $t = T_0 + 1, \ldots, T$, consider the null hypothesis

$H_0 : \eta_t = \eta_{0t}$. Under $H_0$, the potential outcome in the absence of treatment is identified as $Y_t(0) = Y_t - \beta_{0t}$, such that $Y_1, \ldots, Y_{T_0}, Y_t - \beta_{0t}$ could be used to estimate the SC weights $\alpha_{i,i\in\mathcal{D}}$. We define the estimating function

$$\bar{U}_s(\alpha_{i,i\in\mathcal{D}}) = \begin{cases} U_s(\alpha_{i,i\in\mathcal{D}}) = g(Z_s)(Y_s - \sum_{i\in\mathcal{D}} \alpha_i W_{is}) & \text{if } s \leq T_0 \\ g(Z_t)(Y_t - \beta_{0t} - \sum_{i\in\mathcal{D}} \alpha_i W_{it}) & \text{if } s = T_0 + 1 \end{cases}$$

Then $\bar{U}_s(\alpha_{i,i\in\mathcal{D}})$ is an unbiased estimating function for $\alpha_{i,i\in\mathcal{D}}$ under $H_0$, and thus the SC weights $\alpha_{i,i\in\mathcal{D}}$ can be estimated as

$$\bar{\alpha}_{it,i\in\mathcal{D}} = \arg\min_{\alpha_{i,i\in\mathcal{D}}} \bar{m}(\alpha_{i,i\in\mathcal{D}})^{\intercal}\ \Omega\ \bar{m}(\alpha_{i,i\in\mathcal{D}}),$$

where $\bar{m}(\alpha_{i,i\in\mathcal{D}}) = \sum_{s=1}^{T_0+1} \bar{U}_s(\alpha_{i,i\in\mathcal{D}})/(T_0+1)$.

Compute the residuals $\bar{e} = (\bar{e}_1, \ldots, \bar{e}_{T_0+1})^{\intercal}$ where $\bar{e}_s = Y_s - \sum_{i\in\mathcal{D}} \alpha_i W_{is}$ for $s = 1, \ldots, T_0$ and $\bar{e}_{T_0+1} = Y_t - \beta_{0t} - \sum_{i\in\mathcal{D}} \alpha_i W_{is}$. The p-value is

$$\hat{p}(\beta_{0t}) = 1 - \hat{F}(|\bar{e}_{T_0+1}|), \qquad \text{where } \hat{F}(x) = \frac{1}{T_0+1}\sum_{s=1}^{T_0+1} \mathbb{1}(|\bar{e}_s| < x).$$

Under $H_0$ and Assumption 5 that the residual process is stationary and weakly dependent, Chernozhukov et al. (2021) proved that the $p$-value is approximately unbiased. The $1-a$ pointwise prediction interval for $\eta_t$ is constructed by inverting the above test, i.e.:

$$\mathcal{C}_{1-a}(t) = \{\beta_{0t} : \hat{p}(\beta_{0t}) > a\}.$$

In practice, Chernozhukov et al. (2021) proposed to choose a find grid of candidate values for $\eta_{0t}$.

## A.2 Simulation evaluation of the conformal inference method

We perform a simulation study to illustrate the performance of the conformance inference method for pointwise prediction intervals combined with the proposed proximal inference approach. We generate the data under the classical setting identical to that in Section 4 but set $T_1 = 1$. We evaluate the average length and coverage rate of the 90% prediction intervals for $Y_{T_0+1}(1) - Y_{T_0-1}(0) = \beta_{T_0+1}$ over 2,000 Monte Carlo samples.

Table 1 shows the average lengths and coverage probability of the resulting prediction intervals. The conformal pointwise prediction intervals are well-calibrated in all settings. They appear to be wider than the confidence intervals for the CATT described in Section 3.2, likely because CATT is estimated by pooling information of multiple post-treatment time points.

| No. control | Without measured covariates ($\xi = 0$) | | | With measured covariates ($\xi = 0.1$) | | |
|---|---|---|---|---|---|---|
| units | 50 | 100 | 200 | 50 | 100 | 200 |
| 2 | 4.93 (91.3%) | 4.75 (90.0%) | 4.70 (89.7%) | 4.87 (89.2%) | 4.71 (90.8%) | 4.67 (90.0%) |
| 6 | 7.73 (90.7%) | 7.07 (90.7%) | 6.79 (89.3%) | 7.73 (89.8%) | 6.88 (89.4%) | 6.70 (89.7%) |
| 10 | 10.85 (90.4%) | 9.14 (90.4%) | 8.50 (90.8%) | 9.53 (90.2%) | 8.62 (90.3%) | 8.30 (89.0%) |

Table 1: Average length and coverage probability of 90% prediction intervals for $\beta_{T_0+1}$ based on the proposed proximal inference method (PI), with a range of number of control units $N = 2, 6,$ or 10 and pre- and post-treatment time period $T_0 = T - T_0 = 50, 100,$ or 200.

## A.3 Pointwise prediction intervals for causal effects of German Reunification on per-capita GDP in West Germany

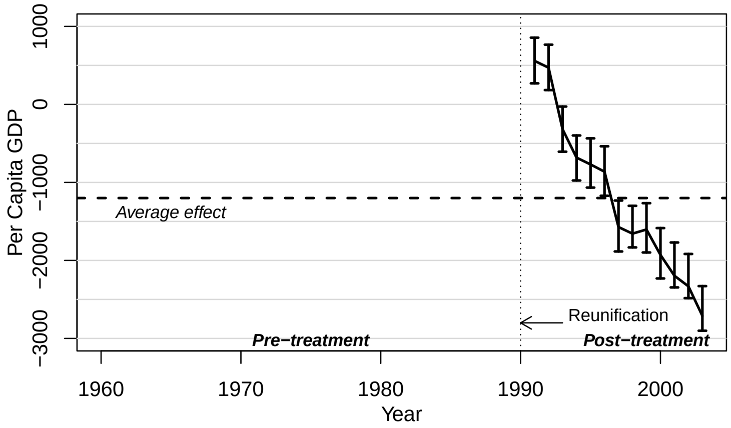


Figure 1: 90% pointwise prediction intervals for causal effects on per-capita GDP in West Germany post reunification. The solid line indicates the difference between per-capita GDP of West Germany and the SC unit constructed by the proximal inference approach described in Section 5.

# B Proof of Theorem 1

Let $A.k$ denote Assumption $k$ for an integer $k$. We first show that

$$E[Y_t(a)] = E[\mathbb{1}(t > T_0)a\beta_t + \sum_{i \in \mathcal{D}} \alpha_i W_{it}]$$

for any $a = 0, 1$ and any $t$. Under Assumptions 1-3 we have

$$Y_t(a) \overset{A.1,A.2}{=} \mathbb{1}(t > T_0)a\beta_t + \mu_0^\intercal \lambda_t + \varepsilon_{0t} \tag{S.1}$$

$$\overset{A.3}{=} \mathbb{1}(t > T_0)a\beta_t + \sum_{i \in \mathcal{D}} \alpha_i W_{it} + \varepsilon_{0t} - \sum_{i \in \mathcal{D}} \alpha_i \varepsilon_{it}, \tag{S.2}$$

for $a = 0, 1$ and any $t$. By Assumption 2, $E[\varepsilon_{it}] = 0$ for any $i, t$, thus we have

$$E[Y_t(a)] \overset{\text{Eq. } (S.2),A.2}{=} E[\mathbb{1}(t > T_0)a\beta_t + \sum_{i \in \mathcal{D}} \alpha_i W_{it}] \tag{S.3}$$

for $a = 0, 1$ and any $t$. In Equation (S.3), setting $a = 0$ we have $E[Y_t(0)] = E[\sum_{i \in \mathcal{D}} \alpha_i W_{it}]$ for any $t$, that is, under Assumptions 1-2, any $\alpha_{i,i \in \mathcal{D}}$ that satisfy Assumption 3 also satisfies $E[Y_t(0)] = E[\sum_{i \in \mathcal{D}} \alpha_i W_{it}]$. Therefore, for any $t > T_0$ we have

$$E[Y_t(1) - Y_t(0)] \overset{A.1}{=} E[Y_t - Y_t(0)] = E[Y_t - \sum_{i \in \mathcal{D}} \alpha_i W_{it}].$$

In Equation (S.3) setting $a = 1$ we have

$$E[Y_t(1)] = beta_t + E[\sum_{i \in \mathcal{D}} \alpha_i W_{it}] = \tau_t + E[\sum_{i \in \mathcal{D}} \alpha_i W_{it}]$$

for any post-treatment period $t > T_0$. Therefore the ATT at time $t > T_0$ is

$$E[Y_t(1) - Y_t(0)] = \tau_t.$$

# C Adjustment for measured covariates

In practice, one may wish to incorporate available covariate data measured across units and over time, either to account for endogeneity or to improve efficiency. Thus we generalize Assumption 2 as follows

**Assumption 2″.** *For any unit $i$ at time $t$,*

$$Y_t = \begin{cases} \tau_t + \mu_0^\intercal \lambda_t + C_{0t}^\intercal \xi_0 + \varepsilon_{0t} & \text{if } t > T_0 \\ \mu_0^\intercal \lambda_t + C_{0t}^\intercal \xi_0 + \varepsilon_{0t} & \text{if } t \le T_0 \end{cases} \tag{S.4}$$

$$W_{it} = \mu_i^\intercal \lambda_t + C_{it}^\intercal \xi_i + \varepsilon_{it},$$

*where $\tau_t$ is the time-varying treatment effects and assumed to be fixed, $C_{it} \in \mathcal{R}^p$ is a $p \times 1$ vector of measured covariates, $\xi_i \in \mathcal{R}^p$ is a $p \times 1$ vector of coefficients, and the error terms satisfy $E[\varepsilon_{it} \mid \lambda_t, C_{it}] = E[\varepsilon_{it}] = 0$ for all $i = 0, \ldots, N$ and $t$.*

In the special case where $\tau_t = \tau$ and $\xi_i = \xi$ for all $t = T_0 + 1, \ldots, T$ and $i = 0, 1, \ldots, N$, Assumption 2″ is the same model considered by Xu (2017).

We modify Assumption 4 to further include $C_t$ as potential common causes of treatment assignment and outcome.

**Assumption 4″.** *We have observed $Z_t$ such that $Z_t \perp\!\!\!\perp (Y_t, W_{it, i \in \mathcal{D}}) \mid C_t, \lambda_t$ for any $t \le T_0$.*

Let $\widetilde{Y}_t = Y_t - C_{0t}^\intercal \xi_0$ and $\widetilde{W}_{it} = W_{it} - C_{it}^\intercal \xi_i$, $i = 1, \ldots, N$. In Corollary 1 below, we state the identification results for $\tau_t$ in the presence of measured covariates corresponding to Theorems 1 and 2:

**Corollary 1** (Identification in the presence of measured covariates)**.**

*(a) Under Assumptions 1, 2′ and 3, we have* $E[Y_t(0)] = E[C_{0t}^{\intercal}\xi_0 + \sum_{i\in\mathcal{D}} \alpha_i \widetilde{W}_{it}]$ *for any* $t$, *and the ATT at time* $t$ *for any* $t \geq T_0$ *is*

$$\tau_t = E[\widetilde{Y}_t - \sum_{i\in\mathcal{D}} \alpha_i \widetilde{W}_{it}]. \tag{S.5}$$

*(b) Under Assumptions 1, 2′, 3 and 4,* $\alpha_{i,i\in\mathcal{D}}$ *and* $\xi_i$ *satisfy the moment condition*

$$E[\widetilde{Y}_t - \sum_{i\in\mathcal{D}} \alpha_i \widetilde{W}_{it} \mid Z_t, C_t] = 0, \quad \forall t \leq T_0.$$

**Example 1′.** *Continuing with Example 1, where the outcomes of control unit(s) not included in the donor pool* $W_{jt,j\in[N]\setminus\mathcal{D}}$ *are selected as supplemental proxy variable* $Z_t$. *We have the following estimating function*

$$U_{PI,t}(\alpha_{i,i\in\mathcal{D}}, \xi_0, \xi_{i,i\in\mathcal{D}}) = g(W_{jt,j\in[N]\setminus\mathcal{D}}, C_t)\left(\widetilde{Y}_t - \sum_{i\in\mathcal{D}} \alpha_i \widetilde{W}_{it}\right),\ t = 1, \ldots, T_0, \tag{S.6}$$

*where* $g(\cdot)$ *is a* $[|\mathcal{D}| + (|\mathcal{D}| + 1)p]$*-dimensional vector of user-specified functions. One can show that* $E[U_{PI,t}(\alpha_{i,i\in\mathcal{D}}, \xi_0, \xi_{i,i\in\mathcal{D}})] = 0$ *for any* $t \leq T_0$.

Furthermore, if the matrix $E[g(W_{jt,j\in[N]\setminus\mathcal{D}}, C_t)(W_{it,i\in\mathcal{D}}, C_{0t}, C_{it,i\in\mathcal{D}})]$ is full row rank, then both the SC weights $\alpha_{i,i\in\mathcal{D}}$ and the coefficients $(\xi_{0t}, \xi_{it,i\in\mathcal{D}})$ can be uniquely identified. When the number of measured covariates is large relative to $T_0$, the resulting estimator may have high variation or even multiple solutions. In such cases, one possible strategy is to assume that measured covariates have the same impact for every unit, i.e. $\xi_i = \xi$ for all $i = 1, \ldots, N$ (Xu 2017) and estimate $(\alpha_{i,i\in\mathcal{D}}, \xi)$ by using the following unbiased estimating function

$$U_{PI,t}(\alpha_{i,i\in\mathcal{D}},\xi) = g(\widetilde{W}_{jt,j\in[N]\setminus\mathcal{D}})\left(\widetilde{Y}_t - \sum_{i\in\mathcal{D}}\alpha_i\widetilde{W}_{it}\right),\ t=1,\ldots,T_0, \tag{S.7}$$

Similar to Section 3.2, one may first infer $\alpha_{i,i\in\mathcal{D}}$ and $\xi_i$ using GMM, then one may implement a standard time series analysis of the corresponding estimate of $e_t = \widetilde{Y}_t - \sum_{i\in\mathcal{D}}\alpha_i\widetilde{W}_{it} = \tau_t + r_t$ to obtain inference about the treatment effect as a function of $t$. Under the CATT model, i.e., $\tau_t = \tau$, an alternative approach is to jointly estimate $\theta = (\alpha_{i,i\in\mathcal{D}},\xi_0,\xi_{i,i\in\mathcal{D}},\tau)$ using GMM; details are omitted but easily inferred from the exposition.

Finally, we extend the above results to the general nonlinear setting, similar to Section 3.3. Below, we modify Assumption $3'$ to incorporate measured covariates:

**Assumption $3'''$.** *There exist a function $h(W_{it,i\in\mathcal{D}}(0),C_t)$ such that the outcome model for $Y_t(0)$ is equivalent to a model for $h(W_{it,i\in\mathcal{D}}(0),C_t)$ had the treatment:*

$$E[Y_t(0)\mid\lambda_t,C_t] = E[h(W_{it,i\in\mathcal{D}}(0),C_t)\mid\lambda_t,C_t],\quad \forall t\le T_0. \tag{S.8}$$

We have the following identification results:

**Corollary 2** (Nonparametric dentification in the presence of measured covariates)**.**

*(a) Under Assumptions 1, $2'$ and $3'''$, we have $E[Y_t(0)] = E[h(W_{it,i\in\mathcal{D}},C_t)]$ for any $t$, and the ATT at time $t$ for any $t\ge T_0$ is*

$$\tau_t = E[Y_t - h(W_{it,i\in\mathcal{D}},C_t)]. \tag{S.9}$$

*(b) Under Assumptions 1, $2'$, $3''$ and $4''$, $h(\cdot)$ satisfy the moment condition*

$$E[Y_t - h(W_{it,i\in\mathcal{D}},C_t)\mid Z_t,C_t] = 0,\quad \forall t\le T_0.$$

Under Model (S.4), it is easy to verify that

$$h(W_{it,i\in\mathcal{D}}, C_t) = \sum_{i\in\mathcal{D}} \alpha_i (W_{it} - C_{it}^{\intercal}\xi_i) + C_{0t}^{\intercal}\xi_0.$$

Estimation and inference of the confounding bridge function and treatment effects are similar to before.

# D Proof of unbiasedness of Eqs. (13) and (16) and Theorem 3

Let $A.k$ denote Assumption $k$ and $T.k$ denote Theorem $k$ for an integer $k$. We first show that $E[U_t(\alpha)] = 0,\ t \leq T_0$ and $E[\widetilde{U}_t(\theta)] = 0$ at the true value under Assumptions 1, 2, 3 and 4. Under these assumptions, $\alpha_{i,i\in\mathcal{D}}$ satisfies $E[Y_t - \sum_{i\in\mathcal{D}} \alpha_i W_{it} \mid Z_{it}] = 0$ for any $t \leq T_0$ by Theorem 2. Therefore, for $t \leq T_0$ we have

$$\begin{aligned} E[U_t(\alpha_{i,i\in\mathcal{D}})] = &\ E\left[g(Z_t)\left(Y_t - \sum_{i\in\mathcal{D}} \alpha_i W_{it}\right)\right] \\ = &\ E\left[g(Z_t) E[Y_t - \sum_{i\in\mathcal{D}} \alpha_i W_{it} \mid Z_t]\right] \\ \overset{T.2}{=} &\ 0 \end{aligned} \tag{S.10}$$

and

$$\begin{aligned} E[\widetilde{U}_t(\theta)] = &\ \begin{pmatrix} E[U_t(\alpha_{i,i\in\mathcal{D}})] \\ 0 \end{pmatrix} \\ \overset{\text{Eq. } (S.10)}{=} &\ 0. \end{aligned} \tag{S.11}$$

For $t > T_0$, we have

$$\begin{aligned} E[\widetilde{U}_t(\theta)] = &\ \begin{pmatrix} 0 \\ E[Y_t - \tau_t - \sum_{i\in\mathcal{D}} \alpha_i W_{it}] \end{pmatrix} \\ \overset{T.1}{=} &\ 0. \end{aligned} \tag{S.12}$$

Now we focus on proving Theorem 3. We follow Chapter 3 of Hall (2005) to prove the asymptotic normality of our estimator. To summarize, we have a population moment condition $E[\widetilde{U}_t(\theta)] = 0$ with a moment function given by Eq. (16), where $\theta = (\alpha_{i,i\in\mathcal{D}}{}^{\intercal}, \tau)^{\intercal} \in \mathcal{R}^{1+|\mathcal{D}|}$. Let $\mathcal{O}_t = \{X_t, Y_t, Z_t^{\intercal}, W_{it,i\in\mathcal{D}}{}^{\intercal}\} \in \mathcal{R}^{2+\dim(Z_t)+|\mathcal{D}|}$ denote the observable vector of random variables, where $\dim(Z_t)$ is the dimension of $Z_t$. Let $\Theta \subseteq \mathcal{R}^{1+|\mathcal{D}|}$ denote the parameter space of $\theta$, and let $O \subseteq \mathcal{R}^{2+\dim(Z_t)+|\mathcal{D}|}$ denote the sample space of $\mathcal{O}_t$. Then $\widetilde{U}_t = \widetilde{U}_t(\mathcal{O}_t; \theta)$ is a mapping from $O \times \Theta$ to $\mathcal{R}^{1+d}$. We impose the following regularity conditions.

**Assumption D.1** (Strict stationarity)**.** *The observable vector of random variables $\mathcal{O}_t$ form a strictly stationary process, such that all expectations of functions of $\mathcal{O}_t$ do not depend on time.*

**Assumption D.2** (Regularity conditions for $\widetilde{U}_t$)**.** *The function $\widetilde{U}_t : O \times \Theta \to \mathcal{R}^{1+d}$ where $d < \infty$ satisfies: (i) it is continuous on $\Theta$ for each $\mathcal{O}_t \in O$; (ii) $E[\widetilde{U}_t(\mathcal{O}_t; \theta)]$ exists and is finite for every $\theta \in \Theta$; (iii) $E[\widetilde{U}_t(\mathcal{O}_t; \theta)]$ is continuous on $\Theta$.*

**Assumption D.3** (Regularity conditions on $\partial\widetilde{U}_t(\mathcal{O}_t; \theta)/\partial\theta'$)**.** *(i) The derivative matrix $\partial\widetilde{U}_t(\mathcal{O}_t; \theta)/\partial\theta'$ exists and is continuous on $\Theta$ for each $\mathcal{O}_t \in O$; (ii) The true value of $\theta$ does not lie on the boundary of $\Theta$; (iii) $E[\partial\widetilde{U}_t(\mathcal{O}_t; \theta)/\partial\theta']$ exists and is finite.*

It is straightforward to verify that Assumption D.2(i) and (iii) and Assumption D.3(i) hold under Assumptions 2-4 due to linearity, although this might not hold under a nonlinear model.

**Assumption D.4** (Properties of the Weighting Matrix)**.** *The user-specified weight matrix $\Omega$ is a positive semi-definite matrix, possibly depends on data, and converges in probability to the positive definite matrix of constants.*

Assumption D.1 is insufficient to allow the application of Laws of Large Numbers and Central Limit Theorem. Therefore we impose the following assumption.

**Assumption D.5** (Ergodicity)**.** *The random process* $\{\mathcal{O}_t; -\infty < t < \infty\}$ *is ergodic.*

**Assumption D.6** (Compactness of $\Theta$)**.** $\Theta$ *is a compact set.*

**Assumption D.7** (Domination of $\widetilde{U}_t(\mathcal{O}_t;\theta)$)**.** $E[\sup_{\theta\in\Theta} \|\widetilde{U}_t(\mathcal{O}_t;\theta)\|] < \infty$.

**Assumption D.8** (Properties of the variance of the sample moment)**.** *Let* $\theta^* = (\gamma^*, \alpha^*)$ *denote the true value of* $\theta$*. (i)* $E[\widetilde{U}_t(\mathcal{O}_t;\theta^*)\widetilde{U}_t(\mathcal{O}_t;\theta^*)^\intercal]$ *exists and is finite; (ii)* $S$ *exists and is a finite valued positive definite matrix.*

**Assumption D.9** (Properties of $G_T(\theta) = T^{-1}\sum_{t=1}^{T} \partial\widetilde{U}_t(\mathcal{O}_t;\theta)/\partial\theta'$)**.** *(i)* $E[\partial\widetilde{U}_t(\mathcal{O}_t;\theta)/\partial\theta']$ *is continuous on some neighbourhood* $N_\epsilon$ *of the true value* $\theta^*$ *in* $\Theta$*; (ii) Uniform convergence of* $G_T(\theta)$*:* $\sum_{\theta\in N_\epsilon} \|G_T(\theta) - E[\partial\widetilde{U}_t(\mathcal{O}_t;\theta)/\partial\theta']\| \xrightarrow{p} 0$.

Finally, we assume that the numbers of pre- and post-treatment periods $T_0$ and $T_1$ are roughly at the same magnitude:

**Assumption D.10.** $T_0/T_1 \to \rho \in (0,\infty)$ *as* $T_0$*,* $T_1 \to \infty$*, where* $\rho$ *is a fixed constant.*

Under Assumptions 1-4 and Regularity Conditions D.1-D.10, further assume that the matrix $E[g(Z_t)W_{it,i\in\mathcal{D}}]$ is full row rank so $\alpha_{i,i\in\mathcal{D}}$ can be uniquely identified, we have that Theorem 3 holds by Theorem 3.2 of Hall (2005).

Finally, we consider a general user-specified parametric model for time-varying treatment effects $\tau_t = \tau(t/T;\gamma)$, indexed by a parameter $\gamma$ with dimension $d_\gamma$. We consider estimating

the parameters $\theta = (\alpha^\intercal, \gamma^\intercal)^\intercal$ by GMM with the estimating function

$$\dot{U}_t(\theta) = \begin{pmatrix} \mathbb{1}(t \leq T_0) g_1(Z_t)(Y_t - \sum_{i\in\mathcal{D}} \alpha_i W_{it}) \\ \mathbb{1}(t > T_0) g_2(t)[Y_t - \tau(t/T;\gamma) - \sum_{i\in\mathcal{D}} \alpha_i W_{it}] \end{pmatrix}$$
$$= \begin{pmatrix} \mathbb{1}(t \leq T_0) g_1(Z_t) \\ \mathbb{1}(t > T_0) g_2(t) \end{pmatrix} [Y_t - \tau(t/T;\gamma) - \sum_{i\in\mathcal{D}} \alpha_i W_{it}], \tag{S.13}$$

where $g_1$ and $g_2$ are real functions with dimensions $d$ and $d_\gamma$, respectively.

We can similarly show that $E[\dot{U}_t(\theta)] = 0$. Furthermore, Let $\dot{\mathcal{D}}_t = \{W_{it,i\in\mathcal{D}}{}^\intercal, \mathbb{1}(t > T_0)[\partial\tau(t/T;\gamma)/\partial\gamma]^\intercal\}^\intercal \in \mathcal{R}^{|\mathcal{D}|+d_\gamma}$, $\dot{\mathcal{V}}_t = \{\mathbb{1}(t \leq T_0) g_1(Z_t)^\intercal, \mathbb{1}(t > T_0) g_2(t)\}^\intercal \in \mathcal{R}^{d+d_\gamma}$, and $\dot{\Omega}$ is a $(d + d_\gamma) \times (d + d_\gamma)$ weighting matrix whose upper-left submatrix equals $\Omega$, lower-right submatrix is symmetric and positive-definite, and the rest entries equal zero. Again, under Assumptions 1-5 with $\tau_t = \tau(t/T;\gamma)$, regularity conditions D.1-D.10, the condition that the matrix $E[g_1(Z_t)W_{it,i\in\mathcal{D}}]$ is full row rank for any $t \leq T_0$, and the condition that the matrix $g_2(t)[\partial\tau(t/T;\gamma)/\gamma]^T$ is full row rank for any $t > T_0$ and $\gamma$ in a neighborhood of the true value, the resulting estimator $\widehat{\theta}$ satisfies

$$\sqrt{T}(\widehat{\theta} - \theta) \xrightarrow{d} N(0, \dot{\Sigma}) \text{ as } T \to \infty,$$

where

$$\dot{\Sigma} = \dot{\Sigma}_0 \dot{S} \dot{\Sigma}_0^\intercal,$$

in which $\dot{S} = \lim_{T\to\infty} Var[\sum_{t=1}^T \dot{U}_t(\theta)/\sqrt{T}]$ is the variance-covariance matrix of the limiting

distribution of $\dot{U}_t(\theta)/\sqrt{T}$, and

$$\dot{\Sigma}_0 = (E[\dot{\mathcal{V}}_t \dot{\mathcal{D}}_t^\intercal]^\intercal \dot{\Omega} E[\dot{\mathcal{V}}_t \dot{\mathcal{D}}_t^\intercal])^{-1} E[\dot{\mathcal{V}}_t \dot{\mathcal{D}}_t^\intercal]^\intercal \dot{\Omega}.$$

We omit the proof as it can easily be inferred from that for Theorem 3.

# E A nonparametric proximal SC estimator

In Theorem 4, we stated that ATT can be identified even when there are multiple confounding bridge functions $h$. In the presence of multiple solutions, one strategy to proceed with inference is to select an optimal estimator that satisfies pre-specified criteria. In this section we present a nonparametric series estimator based on recent methods developed in Santos (2011) and Li et al. (2021), omitting technical proofs and regularity conditions. A manuscript about the general method and theoretic framework in the setting of proximal causal inference is under review elsewhere (Zhang et al. 2023). Although we introduce the estimator in the most general nonparametric setting, the method can incorporate parametric confounding bridge functions, as presented in Section 3.2, with simple modification.

Recall that estimation of ATT requires estimating confounding bridge functions as the solutions to

$$E[Y_t - h(W_{it,i\in\mathcal{D}}) \mid Z_t] = 0, \quad \forall t \leq T_0. \tag{S.14}$$

Therefore we first consider estimating the solution set of Equation (S.14). Let $\mathcal{H}$ be a prespeficied set of smooth functions. Define the solution sets of Equation (S.14) as

$$\mathcal{H}_0 = \{h \in \mathcal{H} : E[h(W_{it,i\in\mathcal{D}}) \mid Z_t] = E[Y_t \mid Z_t], \quad \forall t \leq T_0\}. \tag{S.15}$$

Under the assumptions from Theorem 4, the ATT can be identified as $\tau_t = E[Y_t - h(W_{it,i\in\mathcal{D}})]$ for any $t > T_0$. Under these assumptions, to estimate $\tau_t$, we first construct a consistent estimator $\widehat{\mathcal{H}}_0$ for the set $\mathcal{H}_0$. Next, we select a specific $\hat{h}_0 \in \widehat{\mathcal{H}}_0$ so that it is a consistent estimator for a fixed $h_0 \in \mathcal{H}_0$.

## E.1 Estimation of solution sets

Define a criterion function

$$C(h) = E[E[Y_t - h(W_{it,i\in\mathcal{D}}) \mid Z_t]^2], \quad t \leq T_0.$$

Note that $\mathcal{H}_0 = \{h \in \mathcal{H} : C(h) = 0\}$. We consider a two-stage approach for estimation. We let $\mathcal{H}_n$ be sieve for $\mathcal{H}$, that is, for a known seuence of approximating functions $\{\phi_m(w)\}_{m=1}^{\infty}$, let $\mathcal{H}_n = \{h \in \mathcal{H} : h(w) = \sum_{m=1}^{m_n} \tau_m \phi_m(w)\}$ for an unknown constant $\tau_m$ and a prespecified constant $m_n$. $\mathcal{H}_n$ may also be defined as a parametric model. To construct a sample analogue $C_n$ of $C$, we let $\{\psi_k(z)\}_{k=1}^{\infty}$ be a known sequence of approximating functions. Denote

$$\psi(z) = \{\psi_1(z), \ldots, \psi_{k_n}(z)\}^{\intercal}$$

and let $\Psi = \{\psi(Z_1), \ldots, \psi(Z_{T_0})\}^{\intercal}$. We estimate $E[Y_t \mid Z_t = z_t]$ and $E[h(W_{it,i\in\mathcal{D}}) \mid Z_t = z_t]$ respectively with

$$\hat{E}[Y_t \mid Z_t = z_t] = \psi(z_t)(\Psi^{\intercal}\Psi)^{-1} \sum_{t'=1}^{T_0} \psi(Z_{t'}) Y_{t'}$$

and

$$\hat{E}[h(W_{it,i\in\mathcal{D}}) \mid Z_t = z_t] = \psi(z_t)(\Psi^{\intercal}\Psi)^{-1} \sum_{t'=1}^{T_0} \psi(Z_{t'}) h(W_{it',i\in\mathcal{D}})$$

We then estimate $C(h)$ by

$$C_n(h) = \frac{1}{n} \sum_{t=1}^{T_0} \hat{e}^2(Z_t, h)$$

where $\hat{e}(Z_t, h) = \hat{E}[Y_t \mid Z_t] - \hat{E}[h(W_{it,i\in\mathcal{D}}) \mid Z_t]$.

## E.2 A representer-based estimator

After obtaining $\widehat{\mathcal{H}_0}$, we select a specific estimator from $\widehat{\mathcal{H}_0}$ that converges to a unique element in $\mathcal{H}_0$. We let $M : \mathcal{H} \to \mathbb{R}$ be a population criterion function that attains a unique minimum $h_0$ on $\mathcal{H}_0$ and let $M_n(h)$ be its sample analogue. We then select $\hat{h}_0 \in \operatorname*{argmin}_{h \in \widehat{\mathcal{H}_0}} M_n(h)$. A possible choice for $M$ and $M_n$ are the squared norm $M(h) = E[h(W_{it,i\in\mathcal{D}})^2]$ and its sample analog $M_n(h) = \dfrac{1}{T_0} \sum_{t=1}^{T_0} h(W_{it,i\in\mathcal{D}})$. For a unique solution $\hat{h}_0$ to be attained, we make the following assumptions:

**Assumption E.1.** *The function set $\mathcal{H}$ is convex; the functional $M : \mathcal{H} \to \mathbb{R}$ is strictly convex and attains a unique minimum at $h_0$ on $\mathcal{H}_0$; its sample analogue $M_n : \mathcal{H} \to \mathbb{R}$ is continuous and $\sup_{h\in\mathcal{H}} |M_n(h) - M(h)| = o_p(1)$.*

With the estimated $\hat{h}_0$, a simple estimator for $\hat{\tau}_t$ is $Y_t - \hat{h}_0(W_{it,i\in\mathcal{D}})$. Inference may be attained by the conformal inference approach in Section A. It is possible to use a parametric model for the treatment effect as in Section 3.2, and an asymptotically normal estimator of the treatment effect may be achieved by de-biasing the resulting estimators.

Similar to Section 3.2, we consider a parametric model for the treatment effect $\tau(t/T; \gamma)$. With a fixed function $\hat{h}_0$, the parameter $\gamma$ may be estimated by solving the equation

$$\frac{1}{T - T_0} \sum_{t=T_0+1}^{T} [Y_t - \tau(t/T; \gamma) - \hat{h}_0(W_{it,i\in\mathcal{D}})] = 0.$$

We make the following representer assumption:

**Assumption E.2.** *There exists a function $g_0 \in \mathcal{H}$ such that $\langle g_0, h\rangle_w := E[E\{g_0(W_{it,i\in\mathcal{D}}) \mid Z_t\}E\{h(W_{it,i\in\mathcal{D}}) \mid Z_t\}]$, $t > T_0$, for all $h \in \bar{\mathcal{H}}$, where $\bar{\mathcal{H}}$ denotes the closure of $\mathcal{H}$.*

Without proof, we stated that assuming stationary, independent errors and under certain

regularity conditions, the resulting estimator $\gamma$ satisfies

$$\sqrt{T_1}(\hat{\gamma}-\gamma_0) = \left(\frac{1}{\sqrt{T_1}}\sum_{t=T_0+1}^{T}\frac{\partial}{\partial\gamma}\tau(t/T;\gamma_0)\right)^{-1}\left\{\frac{1}{\sqrt{T}_1}\sum_{t=T_0+1}^{T}\Big[Y_t - E[Y_t] - h_0(W_{it,i\in\mathcal{D}}) + E[Y_t(0)]\right.$$
$$\left. - E\{g_0(W_{it,i\in\mathcal{D}}) \mid Z_t\} \times (Y_t(0) - h_0(W_{it,i\in\mathcal{D}}))\Big] + \sqrt{T_1}r_n(\hat{h}_0)\right\} + o_p(1)$$

where

$$r_n(\hat{h}_0) = \frac{1}{T_1}\sum_{t=T_0+1}^{T}\hat{E}\{\Pi_n g_0(W_{it,i\in\mathcal{D}}) \mid Z_t\}e'(Z_t,\hat{h}_0)$$

and

$$e'(Z_t,h) = E[Y_t(0) \mid Z_t] - E[h(W_{it,i\in\mathcal{D}}) \mid Z_t].$$

## E.3 A debiased asymptotically normal estimator for $\gamma$

An asymptotic estimator for $\gamma$ and thus $\tau(t/T;\gamma)$ requires estimating the term $r_n(\hat{h}_0)$. We define a new criterion function

$$R(h) = E[E\{h(W_{it,i\in\mathcal{D}}) \mid Z_t\}^2] - 2E[h(W_{it,i\in\mathcal{D}})], \quad h \in \mathcal{H}$$

and its sample analog

$$R_n(h) = \frac{1}{T_1}\sum_{t=T_0+1}^{T}\hat{E}[h(W_{it,i\in\mathcal{D}}) \mid Z_t]^2 - \frac{2}{T_1}\sum_{t=T_0+1}^{T}h(W_{it,i\in\mathcal{D}}), \quad h \in \mathcal{H}.$$

We an then estimate the term $\Pi_n g_0$ by

$$\hat{g} \in \underset{h\in\mathcal{H}_n}{\operatorname{argmin}} R_n(h).$$

We can then construct an estimator for $r_n(\hat{h}_0)$ as

$$\hat{r}_n(\hat{h}_0) = \frac{1}{T_1} \sum_{t=T_0+1}^{T} \hat{E}\{\hat{g}(W_{it,i\in\mathcal{D}}) \mid Z_t\} \hat{e}'(Z_t, \hat{h}_0).$$

Here $\hat{e}'(Z_t, h) = \hat{E}[Y_t(0) \mid Z_t] - \hat{E}[h(W_{it,i\in\mathcal{D}}) \mid Z_t]$, where $\hat{E}[Y_t(0) \mid Z_t]$ and $E[h(W_{it,i\in\mathcal{D}}) \mid Z_t]$ are consistent estimators for $E[Y_t(0) \mid Z_t]$ and $E[h(W_{it,i\in\mathcal{D}}) \mid Z_t]$ respectively.

Let $\{\psi'_k(z)\}_{k=1}^{\infty}$ be a known sequence of approximating functions. Denote

$$\psi'(z) = \{\psi'_1(z), \ldots, \psi'_{k_n}(z)\}^{\intercal}$$

and let $\Psi' = \{\psi'(Z_{T_0+1}), \ldots, \psi'(Z_T)\}^{\intercal}$. We may set

$$\hat{E}[\hat{g}(W_{it,i\in\mathcal{D}}) \mid Z_t = z_t] = \psi'(z_t)(\Psi'^{\intercal}\Psi')^{-1} \sum_{t'=T_0+1}^{T} \psi'(Z_{t'})\hat{g}(W_{it',i\in\mathcal{D}}),$$

$$\hat{E}[Y_t(0) \mid Z_t = z_t] = \psi'(z_t)(\Psi'^{\intercal}\Psi')^{-1} \sum_{t'=1}^{T_0} \psi(Z_{t'})[Y_{t'} - \tau(t'/T, \hat{\gamma})]$$

and

$$\hat{E}[h(W_{it,i\in\mathcal{D}}) \mid Z_t = z_t] = \psi'(z_t)(\Psi'^{\intercal}\Psi')^{-1} \sum_{t'=T_0+1}^{T} \psi(Z_{t'})h(W_{it',i\in\mathcal{D}})$$

An asymptotically normal debiased estimator for $\gamma$ is

$$\hat{\gamma}_{db} = \hat{\gamma} - \left( \frac{1}{\sqrt{T}_1} \sum_{t=T_0+1}^{T} \frac{\partial}{\partial \gamma} \tau(t/T; \hat{\gamma}) \right)^{-1} \hat{r}_n(\hat{h}_0).$$

An asymptotically linear estimator for $\tau(\rho, \gamma)$ ($\rho \in (T_0/T, 1]$) is then $\tau(\rho, \hat{\gamma}_{db})$, of which the inference can be obtained via standard the delta-method.

# F Proof of existence of the confounding bridge function

To simplify notation, for each $t \geq 1$, let $W = W_{it,i\in\mathcal{D}}(0)$, $Y = Y_t(0)$, and $\lambda = \lambda_t$. Then Eq. (17) holds if

$$f(y \mid \lambda) = \int h(w) f(w \mid \lambda) dw, \tag{S.16}$$

which is a Fredholm integral equation of the first kind. Conditions for existence of a solution has been considered in Miao et al. (2018) and Cui et al. (2020). Let $L^2[F(s)]$ denote the space of all square-integrable functions of $s$ with respective to a cumulative distribution function $F(s)$, which is a Hilbert space with inner product $< g, h >= \int_{-\infty}^{\infty} g(s)h(s)dF(s)$. Let $K$ denote the conditional expectation operator $L^2[F(w)] \to L^2[F(\lambda)]$, with $Kh = E[h(w) \mid \lambda]$ for $h \in L^2\{F(w)\}$, and let $(\tau_n, \phi_n, \psi_n)_{n=1}^{\infty}$ denote a singular value decomposition of $K$. We assume the following regularity conditions:

Condition F.1: $\int\int f(w \mid \lambda) f(\lambda \mid w) dw d\lambda < \infty$;

Condition F.2: $\int f^2(y \mid \lambda) f(\lambda) d\lambda < \infty$;

Condition F.3: $\sum_{n=1}^{\infty} | < f(y \mid \lambda), \psi_n > |^2 < \infty$.

Condition F.4: Let $q$ be an square-integrable function. If $\int q(\lambda) f(\lambda \mid w) d\lambda = 0$ almost surely, then $q(\lambda) = 0$ almostly.

Then by Picard's theorem (Kress 1989), there exist a solution to Eq. (S.16), which then satisfies Eq. (17).

# G Proof of Theorems 4 and 5

*Proof of Theorem 4*: Write $f_{\lambda_t}$ as the density function for $\lambda_t$. We show that given the confounding bridge function, the mean potential outcome is $E[Y_t(0)] = E[h(W_{it,i\in\mathcal{D}})]$ $(t \geq 1)$. This is because, for any $t \geq 1$,

$$\begin{aligned} E[Y_t(0) - h(W_{it,i\in\mathcal{D}})] &\overset{A.1,A.2'}{=} E[Y_t(0) - h(W_{it,i\in\mathcal{D}}(0))] \\ &= E\{E[Y_t(0) - h(W_{it,i\in\mathcal{D}}(0)) \mid \lambda_t]\} \\ &\overset{A.3''}{=} 0. \end{aligned} \tag{S.17}$$

It is important to note that to identify the average treatment effect on the treated, one only needs to identify $h(W_{it,i\in\mathcal{D}})$, because $E[Y_t(1)] \overset{A.1}{=} E[Y_t]$ in the post-treatment period. In fact, given $h(W_{it,i\in\mathcal{D}})$, the average treatment effect on the treated unit in the post-treatment period is identified by

$$E[Y_t(1) - Y_t(0)] = E[Y_t - h(W_{it,i\in\mathcal{D}})]. \tag{S.18}$$

*Proof of Theorem 5:* We show that any $h$ that satisfies Assumption 3" also satisfies $E(Y_t \mid Z_t) = E[h(W_{it,i\in\mathcal{D}}) \mid Z_t]$ for all $t \leq T_0$ as follows. For any $t \leq T_0$, we have

$$
\begin{aligned}
E[Y_t \mid Z_t] =& E\{E(Y_t \mid \lambda_t, Z_t) \mid Z_t\} \\
\stackrel{A.4}{=}& E\{E(Y_t \mid \lambda_t) \mid Z_t\} \\
\stackrel{A.1}{=}& E\{E(Y_t(0) \mid \lambda_t) \mid Z_t\} \\
\stackrel{A.3''}{=}& E[E\{h(W_{it,i\in\mathcal{D}}(0)) \mid \lambda_t\} \mid Z_t] \\
\stackrel{A.1}{=}& E[E\{h(W_{it,i\in\mathcal{D}}) \mid \lambda_t\} \mid Z_t] \\
\stackrel{A.4}{=}& E[E\{h(W_{it,i\in\mathcal{D}}) \mid \lambda_t, Z_t\} \mid Z_t] \\
=& E[h(W_{it,i\in\mathcal{D}}) \mid Z_t]
\end{aligned}
$$

Therefore

$$
E[Y_t - h(W_{it,i\in\mathcal{D}}) \mid Z_t] = 0, \quad \forall t \leq T_0. \tag{S.19}
$$

# H Additional discussion on the completeness condition and existence of multiple confounding bridge functions

In Theorem 5, we showed that every function $h$ satisfying Equation (17) also satisfies Equation (18). We shall prove that the reverse is true given the following additional assumptions:

**Assumption H.1** (Latent ignorability)**.** *The joint conditional distribution of* $(Y_t(0), W_{it,i\in\mathcal{D}}(0)) \mid \lambda_t$ *is identical for every* $t \geq 1$.

Intuitively, Assumption H.1 requires that $\lambda_t$ accounts for all common causes of the treatment status at time $t$ and $\{Y_t(0), W_{it,i\in\mathcal{D}}\}$ so that there is no remaining confounding.

**Assumption H.2** (Completeness)**.**

*(a) For any square integrable function $q$, if $E[q(\lambda_t) \mid Z_t] = 0$ almost surely, then $q(\lambda_t) = 0$ almost surely for any $t \leq T_0$.*

*(b) For any square integrable function $q$, if $E[q(W_{it,i\in\mathcal{D}}) \mid Z_t] = 0$ almost surely, then $q(W_{it,i\in\mathcal{D}}) = 0$ almost surely for any $t \leq T_0$.*

Assumption H.2(a) formalizes the requirement that $Z_t$ should be $\lambda_t$-relevant, in the sense that any infinitesimal variation in $\lambda_t$ is captured by variation in $Z_t$ such that no information has been lost through projection of $\lambda_t$ on $Z_t$ in the pre-treatment period, and the same goes for Assumption H.2(b). As noted in Section F of the Supplementary Materials, Assumption H.2(a) in addition to mild regularity conditions constitutes sufficient conditions for the existence of confounding bridge functions. Completeness is a fundamental statistical concept in minimum variance unbiased estimation and hypothesis testing (Lehmann & Scheffé 2012,

Basu 2011) and has recently been used to establish identification condition in a variety of problems such as nonparametric instrumental variable methods (Newey & Powell 2003, Ai & Chen 2003, Chernozhukov & Hansen 2005, Hall & Horowitz 2005, Darolles et al. 2011, D'Haultfoeuille 2011, Chen et al. 2014), measurement error (Hu & Schennach 2008, Carroll et al. 2010, An & Hu 2012), and missing data (Miao & Tchetgen Tchetgen 2016). It holds in a large class of commonly-used models such as exponential families (Newey & Powell 2003) and location-scale families (Mattner 1992, Hu & Shiu 2018), and nonparametric additive models (Darolles et al. 2011, D'Haultfoeuille 2011). Andrews (2017) introduced a broad nonparametric class of bivariate distributions that satisfy completeness. In practice, we recommend to measure a rich set of proxies to make the completeness assumption plausible. We refer the readers to Miao et al. (2020) for a thorough review and discussion on the completeness condition.

We have the following results, first for identification of the set of confounding bridge functions and second for unique identification of a confounding bridge function:

**Corollary 3** (Identification of confounding bridge functions)**.**

*(a) Under Assumptions 1, 4, H.1 and H.2(a), any function satisfying Equation* (18) *is a confounding bridge function that satisfies Equation* (17)*;*

*(b) Under Assumptions 1, 4, and Assumption H.2(b), there is a unique confounding bridge function that is identified by solving Equation* (18)*.*

*Proof.* (a) Suppose a function $h$ satisfies Equation (18), then for any $t \leq T_0$,

$$
\begin{aligned}
0 &= E[Y_t - h(W_{it,i\in\mathcal{D}}) \mid Z_t] \\
&= E[E\{Y_t - h(W_{it,i\in\mathcal{D}}) \mid Z_t, \lambda_t\} \mid Z_t] \\
&\overset{A.4}{=} E[E\{Y_t - h(W_{it,i\in\mathcal{D}}) \mid \lambda_t\} \mid Z_t]
\end{aligned}
$$

By Assumption H.2(a), we have $E[Y_t - h(W_{it,i\in\mathcal{D}}) \mid \lambda_t] = 0$ almost surely for any $t \leq T_0$. By Assumption 1, this is equivalent to $E[Y_t(0) - h(W_{it,i\in\mathcal{D}}(0)) \mid \lambda_t] = 0$ almost surely for any $t \leq T_0$.

By Assumption H.1, we have that $E[h(W_{it,i\in\mathcal{D}}(0)) \mid \lambda_t] = E[Y_t(0) \mid \lambda_t]$ almost surely for any $t \geq 1$, i.e., the function $h$ satisfies Equation (17).

(b) Let $h$ be a confounding bridge function. We first show the uniqueness of the solution to Equation (18). By Theorem 5, the function satisfies Equation (18). Suppose that both $h(W_{it,i\in\mathcal{D}})$ and $h'(W_{it,i\in\mathcal{D}})$ satisfy (18) but $h \neq h'$, then we have that $E[h(W_{it,i\in\mathcal{D}}) - h'(W_{it,i\in\mathcal{D}}) \mid Z_t] = 0$ almost surely. By Assumption H.2(b), it must be that $h' = h$ almost surely, which leads to a contradiction. Next, we show the uniqueness of the confounding bridge function. Suppose there is another confounding bridge function $h''$. Then by Theorem 5, the function $h''$ also satisfies Equation (18), which leads to a contradiction. Therefore, the confounding bridge function is unique and is a unique solution to Equation (18).

□

# I Additional simulation studies

## I.1 Weakly dependent errors

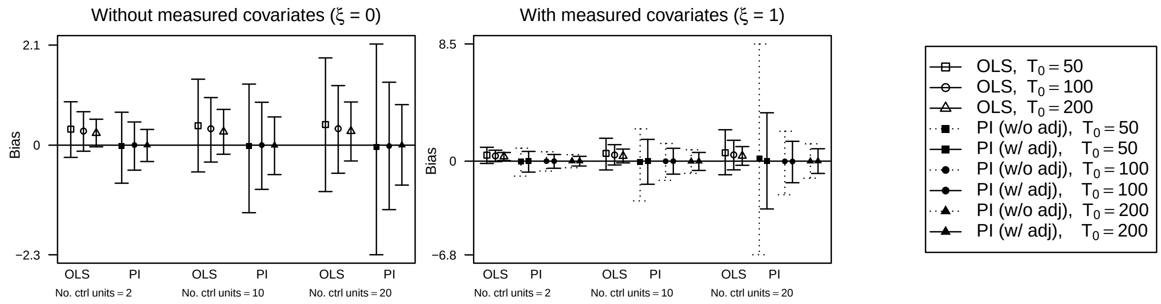


Figure 2: Bias and 95% Monte Carlo confidence interval of the $\tau$ estimates based on the unconstrained regression method (OLS) and our proposed proximal inference method (PI), with a range of number of control units $N = 2, 10,$ or 20 and pre- and post-treatment time period $T_0 = T - T_0 = 50, 100,$ or 200.

| No. | Without measured covariates | | | | | | With measured covariates | | | | | |
|---|---|---|---|---|---|---|---|---|---|---|---|---|
| control | OLS | | | PI | | | OLS | | | PI | | |
| units | 50 | 100 | 200 | 50 | 100 | 200 | 50 | 100 | 200 | 50 | 100 | 200 |
| 2 | 74.4% | 67.3% | 57.6% | 88.9% | 92.3% | 94.3% | 65.2% | 54.5% | 38.4% | 89.3% | 92.5% | 93.3% |
| 10 | 83.8% | 79.3% | 74.7% | 91.1% | 92.7% | 94.4% | 79.7% | 75.6% | 68.4% | 91.1% | 93.8% | 93.6% |
| 20 | 87.1% | 85.5% | 81.6% | 94.3% | 93.7% | 94.9% | 85.5% | 82.6% | 77.6% | 97.3% | 94.3% | 94.3% |

Table 2: Coverage probability based on the unconstrained regression method (OLS) and our proposed proximal inference method (PI), with a range of number of control units $N = 2, 6,$ or 10 and pre- and post-treatment time period $T_0 = T - T_0 = 50, 100,$ or 200.

We present the simulation results bias, variance, and coverage probability in Figure 2 and Table 2 when $\varepsilon_{it}$ is AR(1) with coefficient 0.1, i.e., $\varepsilon_{it} = 0.1\varepsilon_{i,t-1} + \nu_{it}$ where $\nu_{it} \overset{i.i.d}{\sim} N(0, 1)$.

## I.2 Time-varying treatment effect

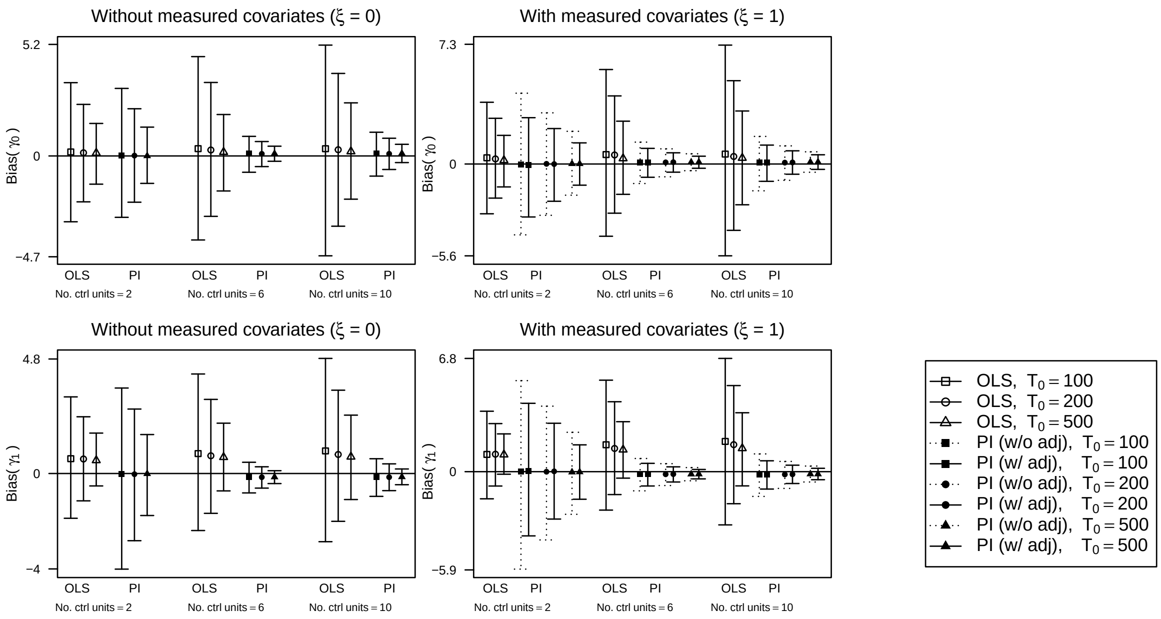


Figure 3: Bias and 95% Monte Carlo confidence interval of the $\gamma_0$ (first row) and $\gamma_1$ (second row) estimates based on the unconstrained regression method (OLS) and our proposed proximal inference method (PI), with a range of number of control units $N = 2, 6,$ or 10 and pre- and post-treatment time period $T_0 = T - T_0 = 100, 200,$ or 500.

| Estimation of $\gamma_0$ | | | | | | | | | | | | |
|---|---|---|---|---|---|---|---|---|---|---|---|---|
| No. | Without measured covariates ($\xi = 0$) | | | | | | With measured covariates ($\xi = 1$) | | | | | |
| control | SC | | | PI | | | SC | | | PI | | |
| units | 100 | 200 | 500 | 100 | 200 | 500 | 100 | 200 | 500 | 100 | 200 | 500 |
| 2 | 91.8% | 88.9% | 94.3% | 93.9% | 94.0% | 94.9% | 88.3% | 80.8% | 63.9% | 94.4% | 93.7% | 95.7% |
| 6 | 91.5% | 89.4% | 85.3% | 100.0% | 100.0% | 100.0% | 87.0% | 83.5% | 69.5% | 100.0% | 100.0% | 100.0% |
| 10 | 91.5% | 91.2% | 87.9% | 100.0% | 100.0% | 100.0% | 87.3% | 84.8% | 77.4% | 100.0% | 100.0% | 100.0% |
| Estimation of $\gamma_1$ | | | | | | | | | | | | |
| No. | Without measured covariates ($\xi = 0$) | | | | | | With measured covariates ($\xi = 1$) | | | | | |
| control | SC | | | PI | | | SC | | | PI | | |
| units | 100 | 200 | 500 | 100 | 200 | 500 | 100 | 200 | 500 | 100 | 200 | 500 |
| 2 | 94.5% | 94.4% | 95.1% | 94.1% | 94.4% | 95.1% | 94.5% | 95.2% | 95.0% | 93.7% | 93.4% | 95.7% |
| 6 | 93.1% | 93.6% | 95.8% | 100.0% | 100.0% | 100.0% | 94.1% | 93.9% | 94.7% | 100.0% | 100.0% | 100.0% |
| 10 | 94.3% | 94.3% | 94.6% | 100.0% | 100.0% | 100.0% | 93.9% | 94.1% | 93.8% | 100.0% | 100.0% | 100.0% |

Table 3: Coverage probability based on the unconstrained regression method (OLS) and our proposed proximal inference method (PI), with a range of number of control units $N = 2, 6,$ or 10 and pre- and post-treatment time period $T_0 = T - T_0 = 100, 200,$ or 500.

We investigate the finite sample performance of our proposed method under various conditions. We simulate time series data on $N$ control units and one treated unit over

$T_0 = 100, 200,$ or 500 time period pre-treatment and the same time length post-treatment, i.e., $T = 2T_0$. We generate samples under the following data generating mechanism

$$Y_t = \begin{cases} \tau(t/T;\gamma) + \mu_0^\intercal \lambda_t + C_{0t}^\intercal \xi + \varepsilon_{0t}, & t > T_0 \\ \mu_0^\intercal \lambda_t + C_{0t}^\intercal \xi + \varepsilon_{0t}, & t \leq T_0 \end{cases}$$

$$W_{it} = \mu_i^\intercal \lambda_t + C_{it}^\intercal \xi + \varepsilon_{it},$$

where $\varepsilon_{it} \overset{i.i.d}{\sim} N(0,2)$ and $\tau(t/T;\gamma) = \gamma_0 + \gamma_1 t/T$ with $\gamma = (1,1)^\intercal$. The rest of the data generating setting is the same as Section 4. We focus on estimation and inference of $\gamma$ using the same approach as detailed in Section 4. Below we present the simulation results in terms of bias, variance, and coverage probability in Figure 3 and Table 3. For estimation of $\gamma_0$, the relative performance comparing OLS and PI methods are similar to Section 4; For estimation of $\gamma_1$, OLS approach still has relatively large bias compared to PI method, although coverage probabilities are closer than the results in Section 4. We also conducted a simulation study when $\varepsilon_{it}$ is AR(1) with coefficient 0.1, i.e., $\varepsilon_{it} = 0.1\varepsilon_{i,t-1} + \nu_{it}$ where $\nu_{it} \overset{i.i.d}{\sim} N(0,1)$. The results are similar to the independent error setting and hence is not shown here.

## I.3 Nonlinear model

| No. control units | Without measured covariates ($\xi = 0$) PI | | | With measured covariates ($\xi = 0.1$) PI (w/ adj) | | |
|---|---|---|---|---|---|---|
| | 500 | 1000 | 5000 | 500 | 1000 | 5000 |
| 2 | 94.99% | 94.73% | 94.50% | 94.87% | 94.75% | 94.07% |
| 4 | 96.25% | 95.95% | 95.48% | 96.45% | 96.68% | 95.21% |
| 6 | 97.45% | 97.44% | 96.71% | 97.61% | 97.86% | 96.80% |

Table 4: Coverage probability based on the unconstrained regression method (OLS) and our proposed proximal inference method (PI), with a range of number of control units $N = 2, 4,$ or 6 and pre- and post-treatment time period $T_0 = T - T_0 = 500, 1000,$ or 5000.

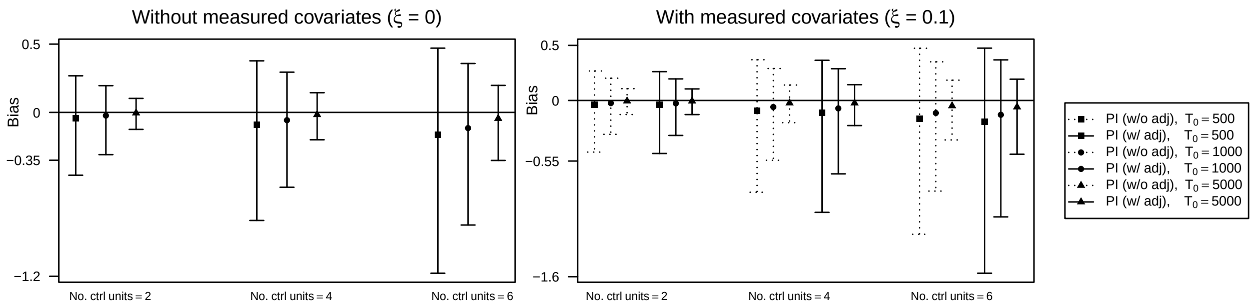


Figure 4: Bias and 95% Monte Carlo confidence interval of the $\beta$ estimates based on the unconstrained regression method (OLS) and our proposed proximal inference method (PI), with a range of number of control units $N = 2, 4,$ or 6 and pre- and post-treatment time period $T_0 = T - T_0 = 500, 1000,$ or 5000.

We investigate the finite sample performance of our proposed method under various conditions. We simulate time series data on $N$ control units and one treated unit over $T_0 = 500, 1000,$ or 5000 time period pre-treatment and the same time length post-treatment, i.e., $T = 2T_0$. We generate $Y_t$ and $W_{it}$ $i = 1, \ldots, N$ from Poisson distribution with

$$E[Y_t \mid X_t, \lambda_t, C_{0t}] = \begin{cases} \exp(\beta + \mu_0^\intercal \lambda_t + C_{0t}^\intercal \xi), & t > T_0 \\ \exp(\mu_0^\intercal \lambda_t + C_{0t}^\intercal \xi), & t \leq T_0 \end{cases} \tag{S.20}$$

$$E[W_{it} \mid \lambda_t, C_{it}] = (\mu_i^\intercal \lambda_t + C_{it}^\intercal \xi)/(e-1),$$

where $X_t = 1$ if $t > T_0$, and $X_t = 0$ otherwise; $C_{it} \overset{i.i.d}{\sim} \text{Uniform}(0,1)$; $\beta = -2$; and $\xi = 0.1$ or 0 corresponding to scenarios with and without measured covariates. We set $\beta$ to $-2$ to avoid extremely large variance of the simulated outcomes due to the mean-variance relationship of Poisson distribution. We simulate a vector of latent factors $\lambda_t = (\lambda_{t1}, \ldots, \lambda_{tr})^\intercal$, where $\lambda_{tk} \overset{i.i.d}{\sim} \text{Uniform}(0,1), k = 1, \ldots, r$, and $r = 1, 2$ or 3. That is, we generate three settings with one, two, or three latent factors. We reduce the number of latent factors compared to previous simulation studies to achieve a more stable result for illustration purpose. For

each setting, we assume the number of control units $N = 2r$, and the first half of the control units ($i = 1, \ldots, r$) constitute the donor pool with $|\mathcal{D}| = r$. We specify factor loadings $\mu_i,\ i = 0, \ldots, N$ as follows

$$\begin{array}{ccccccc} \mu_0 & \mu_1 & \cdots & \mu_r & \mu_{r+1} & \cdots & \mu_{2r} \end{array}$$
$$\begin{pmatrix} 1 & 1 & & & 1 & & \\ \vdots & & \ddots & & & \ddots & \\ 1 & & & 1 & & & 1 \end{pmatrix} \quad \text{for } 2r = N = 2, 4, 6.$$

From the above model we know that $\beta = E[Y_t(1)]/E[Y_t(0)] = -2$. We focus on estimation of $\beta$ in this setting for simplicity. We implement the PI method taking the first half of control units as donors $W_{it,i\in\mathcal{D}}$ and second half of control units as supplemental proxies $W_{jt,j\in[N]\backslash\mathcal{D}}$. When there exists a measured covariate (i.e., $\xi = 0.1$) which is predictive of the outcome, we implement our method with and without covariate adjustment to investigate whether there is an efficiency gain from adjusting for such a predictor of the outcome. From Eq. (S.20), we derived that the confounding bridge function satisfying Assumption 3$'$ is given by

$$h(W_{it,i\in\mathcal{D}}, C_{it,i\in\mathcal{D}}, C_{0t}; \alpha_{i,i\in\mathcal{D}}, \xi) = \exp[\sum_{i\in\mathcal{D}} \alpha_i (W_{it} - C_{it}^{\intercal}\xi) + C_{0t}^{\intercal}\xi].$$

For inference, we compute an estimate of HC variance-covariance matrix as detailed in Section 3.2. Below we present the simulation results in terms of bias, variance, and coverage probability in Figure 4 and Table 4.

# References


Ai, C. & Chen, X. (2003), 'Efficient Estimation of Models with Conditional Moment Restrictions Containing Unknown Functions', *Econometrica* **71**(6), 1795–1843.

An, Y. & Hu, Y. (2012), 'Well-posedness of measurement error models for self-reported data', *Journal of Econometrics* **168**(2), 259–269.

Andrews, D. W. (2017), 'Examples of l2-complete and boundedly-complete distributions', *Journal of econometrics* **199**(2), 213–220.

Basu, D. (2011), On Statistics Independent of a Complete Sufficient Statistic, *in* 'Selected Works of Debabrata Basu', Springer, pp. 61–64.

Carroll, R. J., Chen, X. & Hu, Y. (2010), 'Identification and estimation of nonlinear models using two samples with nonclassical measurement errors', *Journal of Nonparametric Statistics* **22**(4), 379–399.

Chen, X., Chernozhukov, V., Lee, S. & Newey, W. K. (2014), 'Local Identification of Nonparametric and Semiparametric Models', *Econometrica* **82**(2), 785–809.

Chernozhukov, V. & Hansen, C. (2005), 'An IV Model of Quantile Treatment Effects', *Econometrica* **73**(1), 245–261.

Chernozhukov, V., Wüthrich, K. & Zhu, Y. (2021), 'An Exact and Robust Conformal Inference Method for Counterfactual and Synthetic Controls', *Journal of the American Statistical Association* pp. 1–16.

Cui, Y., Pu, H., Shi, X., Miao, W. & Tchetgen Tchetgen, E. J. (2020), 'Semiparametric proximal causal inference', *arXiv preprint arXiv:2011.08411* .

Darolles, S., Fan, Y., Florens, J. P. & Renault, E. (2011), 'Nonparametric Instrumental Regression', *Econometrica* **79**(5), 1541–1565.

D'Haultfoeuille, X. (2011), 'On the Completeness Condition in Nonparametric Instrumental Problems', *Econometric Theory* **27**(3), 460–471.

Hall, A. R. (2005), *Generalized Method of Moments*, Oxford University Press.

Hall, P. & Horowitz, J. L. (2005), 'Nonparametric Methods for Inference in the Presence of Instrumental Variables', *The Annals of Statistics* **33**(6), 2904–2929.

Hu, Y. & Schennach, S. M. (2008), 'Instrumental Variable Treatment of Nonclassical Measurement Error Models', *Econometrica* **76**(1), 195–216.

Hu, Y. & Shiu, J.-L. (2018), 'Nonparametric Identification Using Instrumental Variables: Sufficient Conditions for Completeness', *Econometric Theory* **34**(3), 659–693.

Kress, R. (1989), *Linear Integral Equations*, Vol. 82, Springer.

Lehmann, E. L. & Scheffé, H. (2012), Completeness, Similar Regions, and Unbiased Estimation-Part I and Part II, *in* 'Selected Works of E. L. Lehmann', Springer, pp. 233–286.

Li, W., Miao, W. & Tchetgen, E. T. (2021), 'Identification and estimation of nonignorable missing outcome mean without identifying the full data distribution', *arXiv preprint arXiv:2110.05776* .

Mattner, L. (1992), 'Completeness of location families, translated moments, and uniqueness of charges', *Probability Theory and Related Fields* **92**(2), 137–149.

Miao, W., Geng, Z. & Tchetgen Tchetgen, E. J. (2018), 'Identifying causal effects with proxy variables of an unmeasured confounder', *Biometrika* **105**(4), 987–993.

Miao, W., Hu, W., Ogburn, E. L. & Zhou, X. (2020), 'Identifying effects of multiple treatments in the presence of unmeasured confounding', *arXiv preprint arXiv:2011.04504* .

Miao, W. & Tchetgen Tchetgen, E. J. (2016), 'On varieties of doubly robust estimators under missingness not at random with a shadow variable', *Biometrika* **103**(2), 475–482.

Newey, W. K. & Powell, J. L. (2003), 'Instrumental Variable Estimation of Nonparametric Models', *Econometrica* **71**(5), 1565–1578.

Santos, A. (2011), 'Instrumental variable methods for recovering continuous linear functionals', *Journal of Econometrics* **161**(2), 129–146.

Xu, Y. (2017), ‘Generalized Synthetic Control Method: Causal Inference With Interactive Fixed Effects Models’, *Political Analysis* **25**(1), 57–76.

Zhang, J., Li, W., Miao, W. & Tchetgen Tchetgen, E. (2023), ‘Proximal causal inference without uniqueness assumptions’. Under review.
